# Supplementary material for: Decoder-Only LLMs are Better Controllers for Diffusion Models
Source: arXiv:2502.04412 source file (2025-02-06)
Supplement: Supplementary file 1 [file X_suppl.tex]

\clearpage
\setcounter{page}{1}
\maketitlesupplementary

\section{Cross Language Generation}

\begin{figure}[H]
    \centering
    \includegraphics[width=0.98\textwidth]{imgs_supp/exp_multi_lang.jpg}
    \caption{
    Our method is capable of cross language generation by utilizing the pre-trained knowledge embedded within the multilingual LLM.
    }

    \label{fig:exp_multi_lang}
\end{figure}

We evaluated the cross language generation capabilities of our method based on the chatglm3-6b~\cite{glm} model. chatglm3-6b is an LLM with knowledge of both Chinese and English languages. As illustrated in \cref{fig:exp_multi_lang}, despite solely utilizing English image-text pairs during training, our method is capable of using Chinese prompts for image generation in the inference phase. This indicates that our method effectively leverages the pre-trained knowledge embodied in the LLM.
